# Supplementary material for: Locally-Minimal Probabilistic Explanations
Source: arXiv:2312.11831 source file (2024-05-06)
Supplement: Supplementary file 1 [file appendix.tex]

%\onecolumn
%\title{Title in Title Case\\(Supplementary Material)}
%\maketitle
%\appendix
 
%\vspace{-3.5cm}

\section{Detailed Results}

\subsection{Random Forests}
\sisetup{parse-numbers=false,detect-all,mode=text}
\setlength{\tabcolsep}{5pt}
\let\lpr\undefined
\let\rpr\undefined
\newcommand{\lpr}{(}
\newcommand{\rpr}{)}

\begin{table}[ht]
\centering
\resizebox{0.99\columnwidth}{!}{
  \begin{tabular}{l>{\lpr}S[table-format=2.0,table-space-text-pre=\lpr]S[table-format=2.0,table-space-text-post=\rpr]<{\rpr}
  S[table-format=2.1]S[table-format=2.2]
  S[table-format=2.1]S[table-format=2]S[table-format=1.2]S[table-format=2.2] }
\toprule[1.2pt]
\multirow{2}{*}{\bf Dataset} & \multicolumn{2}{c}{\multirow{2}{*}{\bf (m,~K)}}  & 
\multicolumn{2}{c}{\bf  AXp }  & \multicolumn{4}{c}{\bf  LmPAXp}   \\
\cmidrule[0.8pt](lr{.75em}){4-5}
\cmidrule[0.8pt](lr{.75em}){6-9}
& \multicolumn{2}{c}{}  & {\bf Len }  &  {\bf Time}  &  {\bf Len }  & {\bf \% }  & {\bf Prec }  &  {\bf Time }  \\
\toprule[1.2pt]

adult  &  12  &  2  &  5.6  &  0.19  &  3.2  &  57  &  0.97  &  0.99 \\
agaricus  &  22  &  2  &  10.0  &  0.06  &  3.3  &  33  &  0.96  &  3.78 \\
compas  &  11  &  2  &  5.6  &  0.12  &  3.6  &  64  &  0.97  &  0.77 \\
german  &  21  &  2  &  12.3  &  0.36  &  3.2  &  26  &  0.97  &  5.40 \\
heart-c  &  13  &  2  &  5.5  &  0.07  &  3.0  &  55  &  0.97  &  0.39 \\
ionosphere  &  34  &  2  &  21.5  &  0.06  &  2.9  &  13  &  0.96  &  6.59 \\
kr\_vs\_kp  &  36  &  2  &  8.1  &  0.08  &  3.5  &  43  &  0.98  &  0.84 \\
lending  &  9  &  2  &  2.2  &  0.10  &  1.7  &  77  &  0.99  &  0.15 \\
mofn\_3\_7\_10  &  10  &  2  &  3.1  &  0.06  &  2.8  &  90  &  0.99  &  0.13 \\
mushroom  &  22  &  2  &  9.2  &  0.07  &  4.2  &  46  &  0.97  &  2.30 \\
parity5+5  &  10  &  2  &  6.8  &  0.23  &  6.4  &  94  &  0.99  &  0.38 \\
recidivism  &  15  &  2  &  7.9  &  0.48  &  5.8  &  73  &  0.97  &  1.75 \\
segmentation  &  19  &  7  &  8.1  &  0.39  &  4.9  &  60  &  0.98  &  0.76 \\
soybean  &  35  &  18  &  15.6  &  2.05  &  8.9  &  57  &  0.97  &  4.07 \\
tic\_tac\_toe  &  9  &  2  &  5.0  &  0.09  &  3.3  &  66  &  0.97  &  0.58 \\
twonorm  &  20  &  2  &  10.4  &  0.05  &  4.4  &  42  &  0.97  &  1.35 \\
vote  &  16  &  2  &  5.6  &  0.07  &  2.6  &  46  &  0.98  &  1.16 \\

\bottomrule[1.2pt]
\end{tabular}
}
\caption{%
\footnotesize{
  Detailed performance evaluation of computing LmPAXp for RFs.
The table shows results for 17 datasets containing binary and 
categorical data. The maximum tolerance  was fixed to 0.05, i.e.\ 
$\Tau = 0.95$.
Columns {\bf m} and {\bf K} report, respectively, the
number of features and classes in the dataset.
Columns {\bf Len} and  {\bf Time}  report, resp., the average length 
of computed AXp's (resp.\ LmPAXp) and  the average runtime for computing 
such explanations.
Column {\bf Prec} reports the average precision of the probabilistic explanations.
}}
\label{tab:RFs-sat}
\end{table}

\subsection{Binarized Neural Networks}
\input{texfigs/BNNs-pb}
